# Supplementary material for: Divide & Bind Your Attention for Improved Generative Semantic Nursing
Source: arXiv:2307.10864 source file (2024-07-14)
Supplement: Supplementary file 1 [file attention_vis_2.tex]

\begin{figure*}[t]
\begin{centering}
\setlength{\tabcolsep}{0.0em}

\par\end{centering}
\begin{centering}
%\vspace{-2em}
\hfill{}%
	\begin{tabular}{
    m{1.5em}<{\centering} %@{\hspace{1em}}
    m{0.15\linewidth}<{\centering} @{\hspace{-1em}}
    m{0.15\linewidth}<{\centering}  @{}%@{\hspace{-5em}}
    m{0.15\linewidth}<{\centering} @{}
    m{0.15\linewidth}<{\centering}
    }
    
    &
    \multicolumn{3}{c}{\hspace{4em}\myquote{A \textblue{pineapple} and two \textblue{oranges}  }} 
    
    \tabularnewline
    &
    $x_0$
    & \hspace{3em}$\hat{x_0}^{(t)}$\hspace{-1em}
    & %{\hspace{4em} } %{\footnotesize{}}
    \hspace{0.2em}pineapple
    & %{\footnotesize{}} {\hspace{4em} }
     \hspace{-1em}oranges
	%\vspace{0.02cm} 
    %% Stable Diffsuion
    \tabularnewline
    \multirow{1}{*}{\rotatebox{90}{
        \hspace{2.5em}
        \begin{tabular}{c}
        \small Stable\\ \small Diffusion 
        \end{tabular}
        \hspace{-2.5em}
    }} 
    &
    \includegraphics[height=0.09\textheight]{fig/attn_gif/SD/19_8516_sd.png}
    &
    \multicolumn{3}{c}{\begin{tabular}{c}\animategraphics[autoplay,loop,height=0.09\textheight]{3}{fig/attn_gif/SD/}{0}{50}\end{tabular}} 
    
	 %% Attend and Excite
  \tabularnewline
  \multirow{1}{*}{\rotatebox{90}{
        \hspace{2.4em}
        \begin{tabular}{c<{\centering}}
        \small
        Attend \& \\ \small Excite
        \end{tabular}
        \hspace{-2.4em}
    }} 
    &
    \includegraphics[height=0.09\textheight]{fig/attn_gif/AE/19_8516_excite.png}
    &
    \multicolumn{3}{c}{\begin{tabular}{c}\animategraphics[autoplay,loop,height=0.09\textheight]{3}{fig/attn_gif/AE/}{0}{50}\end{tabular}} 
	 \tabularnewline
  %% Ours
    \multirow{1}{*}{\rotatebox{90}{
        \hspace{3.5em}
        \begin{tabular}{c}
        \small \textbf{Divide \& Bind} \\
        \small (Ours) 
        \end{tabular}
        \hspace{-3.5em}
    }} 
    &
    \includegraphics[height=0.09\textheight]{fig/attn_gif/TV/19_8516_tv-0.05-0.2-0.3-init50.png}
    &
    \multicolumn{3}{c}{\begin{tabular}{c}\animategraphics[autoplay,loop,height=0.09\textheight]{3}{fig/attn_gif/TV/}{0}{50}\end{tabular}} 

    \tabularnewline
	\end{tabular}
\hfill{}
\par\end{centering}
\caption{
Visualization of the cross-attention maps for each subject token [This is a GIF, can be viewed in the downloaded PDF file] \YL{last frame;to be replaced!}
} 
\label{fig:attention_vis_eg1}
%\vspace{-0.7em}
\end{figure*}

%%%%%%%%%%%%%%%%%%%%%%%%%%%%%%%%%%%%%%%%%%%%%
% Some GIF Attempts
%%%%%%%%%%%%%%%%%%%%%%%%%%%%%%%%%%%%%%%%%%%%%
% Version 1
% \begin{figure*}[t]
% \centering
% %\includegraphics[width=0.8\linewidth]
% \animategraphics[autoplay,loop,height=4cm]{7}{fig/gif/test/}{0}{15}
% \caption{GIF works in downloaded Adobe PDF!}
% \label{fig:attn}
% %\vspace{-1.0em}
% \end{figure*}
% Version 1
% \begin{center}
% \animategraphics[autoplay,loop,height=4cm]{7}{fig/gif/test/}{0}{15}
% \end{center}

% Version 2
% \includemedia[width=0.6\linewidth,height=0.6\linewidth,activate=pageopen,
% passcontext,
% transparent,
% addresource=fig/gif/TV-2banana-2oranges-8516.mp4,
% flashvars={source=fig/gif/TV-2banana-2oranges-8516.mp4}
% ]{\includegraphics[width=0.6\linewidth]{fig/dummy_pic_bear.jpg}}{VPlayer.swf}
